# Supplementary material for: High-Resolution Spectroscopy of {R}ydberg Molecular States of $^{85}${R}b$_2$ Near the $5s+7p$ Asymptote
Source: arXiv:1702.05132 ancillary file (2017-04-27)
Supplement: Supplementary file 1 [file fcf_tables.pdf]

## Tables of Franck-Condon Factors

This Supplement contains tables of Franck-Condon factors from the  $a^3\Sigma_u^+$  state to the inner and outer wells of the  $7p^3\Sigma_g^+$  state, with the lower-state potential from Ref. [23] and the upper-state potential from Ref. [15]. These FCFs were calculated using LEVEL 8.2 [22].

Table 1: Franck-Condon Factors from the  $a^3\Sigma_u^+$  state to the inner well of the  $7p^3\Sigma_g^+$  state. Here,  $v'$  is the vibrational quantum number for the full potential, and  $v'$  (inner) is the numbering for the inner well alone.

| $v'$ | $v'$ (inner) | $E(v')$ ( $\text{cm}^{-1}$ ) | FCF $v'' = 35$ | FCF $v'' = 36$ |
|------|--------------|------------------------------|----------------|----------------|
| 0    | 0            | 23650.1503                   | –              | –              |
| 1    | 1            | 23690.77                     | 0.0018         | 0.00116        |
| 2    | 2            | 23731.29                     | 0.00124        | 7.90E-04       |
| 3    | 3            | 23771.62                     | 7.84E-05       | 4.67E-05       |
| 4    | 4            | 23811.77                     | 3.80E-04       | 2.52E-04       |
| 5    | 5            | 23851.8                      | 9.47E-04       | 6.09E-04       |
| 6    | 6            | 23891.69                     | 3.46E-04       | 2.15E-04       |
| 7    | 7            | 23931.44                     | 3.99E-05       | 2.90E-05       |
| 8    | 8            | 23971.04                     | 6.19E-04       | 4.04E-04       |
| 9    | 9            | 24010.51                     | 5.73E-04       | 3.62E-04       |
| 10   | 10           | 24049.87                     | 3.00E-05       | 1.63E-05       |
| 11   | 11           | 24089.11                     | 2.59E-04       | 1.74E-04       |
| 12   | 12           | 24128.24                     | 6.35E-04       | 4.09E-04       |
| 13   | 13           | 24167.26                     | 2.63E-04       | 1.61E-04       |
| 14   | 14           | 24206.18                     | 1.36E-05       | 1.13E-05       |
| 15   | 15           | 24244.98                     | 4.16E-04       | 2.75E-04       |
| 16   | 16           | 24283.67                     | 5.26E-04       | 3.34E-04       |
| 17   | 17           | 24322.26                     | 1.07E-04       | 6.26E-05       |
| 18   | 18           | 24360.74                     | 7.27E-05       | 5.25E-05       |
| 19   | 19           | 24399.11                     | 4.63E-04       | 3.04E-04       |
| 20   | 20           | 24437.37                     | 4.36E-04       | 2.74E-04       |
| 21   | 21           | 24475.52                     | 5.70E-05       | 3.15E-05       |
| 22   | 22           | 24513.55                     | 9.96E-05       | 7.10E-05       |
| 23   | 23           | 24551.45                     | 4.54E-04       | 2.97E-04       |
| 24   | 24           | 24589.24                     | 4.05E-04       | 2.53E-04       |
| 25   | 25           | 24626.89                     | 5.68E-05       | 3.10E-05       |
| 26   | 26           | 24664.41                     | 8.19E-05       | 5.96E-05       |
| 27   | 27           | 24701.8                      | 4.16E-04       | 2.74E-04       |
| 28   | 28           | 24739.04                     | 4.22E-04       | 2.65E-04       |
| 29   | 29           | 24776.15                     | 9.34E-05       | 5.28E-05       |
| 30   | 30           | 24813.11                     | 3.83E-05       | 3.01E-05       |
| 31   | 31           | 24849.92                     | 3.48E-04       | 2.32E-04       |
| 32   | 32           | 24886.59                     | 4.59E-04       | 2.91E-04       |
| 33   | 33           | 24923.1                      | 1.76E-04       | 1.03E-04       |
| 34   | 34           | 24959.47                     | 2.23E-06       | 3.18E-06       |

Continued on next page...

| <b>v'</b> | <b>v' (inner)</b> | <b>E(v') (cm<sup>-1</sup>)</b> | <b>FCF v'' = 35</b> | <b>FCF v'' = 36</b> |
|-----------|-------------------|--------------------------------|---------------------|---------------------|
| 35        | 35                | 24995.68                       | 2.38E-04            | 1.63E-04            |
| 36        | 36                | 25031.75                       | 4.71E-04            | 3.04E-04            |
| 37        | 37                | 25067.66                       | 3.05E-04            | 1.86E-04            |
| 38        | 38                | 25103.42                       | 2.42E-05            | 1.11E-05            |
| 39        | 39                | 25139.02                       | 9.81E-05            | 7.24E-05            |
| 40        | 40                | 25174.48                       | 4.02E-04            | 2.67E-04            |
| 41        | 41                | 25209.79                       | 4.40E-04            | 2.76E-04            |
| 42        | 42                | 25244.95                       | 1.54E-04            | 8.81E-05            |
| 43        | 43                | 25279.96                       | 2.77E-06            | 4.07E-06            |
| 44        | 44                | 25314.82                       | 2.24E-04            | 1.56E-04            |
| 45        | 45                | 25349.52                       | 4.72E-04            | 3.06E-04            |
| 46        | 46                | 25384.07                       | 3.66E-04            | 2.24E-04            |
| 47        | 47                | 25418.47                       | 7.18E-05            | 3.73E-05            |
| 48        | 48                | 25452.71                       | 3.26E-05            | 2.81E-05            |
| 49        | 49                | 25486.81                       | 3.07E-04            | 2.10E-04            |
| 50        | 50                | 25520.76                       | 4.92E-04            | 3.16E-04            |
| 51        | 51                | 25554.55                       | 3.22E-04            | 1.94E-04            |
| 52        | 52                | 25588.2                        | 4.40E-05            | 2.07E-05            |
| 53        | 53                | 25621.69                       | 5.28E-05            | 4.34E-05            |
| 54        | 54                | 25655.03                       | 3.37E-04            | 2.30E-04            |
| 55        | 55                | 25688.22                       | 5.05E-04            | 3.23E-04            |
| 56        | 56                | 25721.25                       | 3.29E-04            | 1.97E-04            |
| 57        | 57                | 25754.14                       | 5.05E-05            | 2.37E-05            |
| 58        | 58                | 25786.87                       | 4.28E-05            | 3.71E-05            |
| 59        | 59                | 25819.44                       | 3.18E-04            | 2.20E-04            |
| 60        | 60                | 25851.87                       | 5.19E-04            | 3.35E-04            |
| 61        | 61                | 25884.14                       | 3.89E-04            | 2.34E-04            |
| 62        | 62                | 25916.25                       | 9.56E-05            | 4.86E-05            |
| 63        | 63                | 25948.21                       | 1.25E-05            | 1.43E-05            |
| 64        | 64                | 25980.01                       | 2.46E-04            | 1.76E-04            |
| 65        | 65                | 26011.66                       | 5.11E-04            | 3.36E-04            |
| 66        | 66                | 26043.14                       | 4.85E-04            | 2.99E-04            |
| 67        | 67                | 26074.47                       | 2.03E-04            | 1.12E-04            |
| 68        | 68                | 26105.65                       | 3.22E-06            | 1.52E-07            |
| 69        | 69                | 26136.66                       | 1.27E-04            | 9.92E-05            |
| 70        | 70                | 26167.51                       | 4.33E-04            | 2.95E-04            |
| 71        | 71                | 26198.2                        | 5.70E-04            | 3.62E-04            |
| 72        | 72                | 26228.72                       | 3.81E-04            | 2.24E-04            |
| 73        | 73                | 26259.08                       | 8.32E-05            | 3.89E-05            |
| 74        | 74                | 26289.28                       | 1.69E-05            | 1.97E-05            |
| 75        | 75                | 26319.31                       | 2.62E-04            | 1.92E-04            |
| 76        | 76                | 26349.17                       | 5.52E-04            | 3.67E-04            |

Continued on next page...

| <b>v'</b> | <b>v' (inner)</b> | <b>E(v') (cm<sup>-1</sup>)</b> | <b>FCF v'' = 35</b> | <b>FCF v'' = 36</b> |
|-----------|-------------------|--------------------------------|---------------------|---------------------|
| 77        | 77                | 26378.86                       | 5.71E-04            | 3.54E-04            |
| 78        | 78                | 26408.38                       | 2.98E-04            | 1.67E-04            |
| 79        | 79                | 26437.73                       | 3.07E-05            | 1.02E-05            |
| 80        | 80                | 26466.91                       | 6.20E-05            | 5.68E-05            |
| 81        | 81                | 26495.91                       | 3.67E-04            | 2.62E-04            |
| 82        | 82                | 26524.74                       | 6.29E-04            | 4.12E-04            |
| 83        | 83                | 26553.39                       | 5.75E-04            | 3.50E-04            |
| 84        | 84                | 26581.86                       | 2.61E-04            | 1.40E-04            |
| 85        | 85                | 26610.14                       | 1.39E-05            | 2.43E-06            |
| 86        | 86                | 26638.24                       | 9.77E-05            | 8.56E-05            |
| 87        | 87                | 26666.15                       | 4.38E-04            | 3.11E-04            |
| 88        | 88                | 26693.88                       | 6.96E-04            | 4.53E-04            |
| 89        | 89                | 26721.41                       | 6.10E-04            | 3.66E-04            |
| 90        | 90                | 26748.75                       | 2.65E-04            | 1.38E-04            |
| 91        | 91                | 26775.9                        | 1.10E-05            | 1.10E-06            |
| 92        | 92                | 26802.84                       | 1.15E-04            | 1.02E-04            |
| 93        | 93                | 26829.57                       | 4.90E-04            | 3.50E-04            |
| 94        | 94                | 26856.1                        | 7.71E-04            | 5.02E-04            |
| 95        | 95                | 26882.42                       | 6.78E-04            | 4.05E-04            |
| 96        | 96                | 26908.53                       | 2.99E-04            | 1.53E-04            |
| 97        | 97                | 26934.42                       | 1.38E-05            | 1.27E-06            |
| 98        | 98                | 26960.09                       | 1.24E-04            | 1.13E-04            |
| 99        | 99                | 26985.54                       | 5.44E-04            | 3.92E-04            |
| 100       | 100               | 27010.75                       | 8.69E-04            | 5.67E-04            |
| 101       | 101               | 27035.73                       | 7.73E-04            | 4.59E-04            |
| 102       | 102               | 27060.47                       | 3.43E-04            | 1.72E-04            |
| 103       | 103               | 27084.97                       | 1.56E-05            | 1.05E-06            |
| 104       | 104               | 27109.22                       | 1.47E-04            | 1.37E-04            |
| 105       | 105               | 27133.22                       | 6.39E-04            | 4.63E-04            |
| 106       | 106               | 27156.96                       | 0.00101             | 6.57E-04            |
| 107       | 107               | 27180.44                       | 8.77E-04            | 5.13E-04            |
| 108       | 108               | 27203.64                       | 3.60E-04            | 1.72E-04            |
| 109       | 109               | 27226.57                       | 6.47E-06            | 2.48E-07            |
| 110       | 110               | 27249.21                       | 2.32E-04            | 2.09E-04            |
| 111       | 111               | 27271.56                       | 8.53E-04            | 6.10E-04            |
| 112       | 112               | 27293.61                       | 0.00123             | 7.80E-04            |
| 113       | 113               | 27315.34                       | 9.28E-04            | 5.19E-04            |
| 114       | 114               | 27336.75                       | 2.64E-04            | 1.06E-04            |
| 115       | 115               | 27357.83                       | 1.42E-05            | 3.67E-05            |
| 116       | 116               | 27378.57                       | 5.55E-04            | 4.52E-04            |
| 117       | 117               | 27398.95                       | 0.00134             | 9.09E-04            |
| 118       | 118               | 27418.96                       | 0.00143             | 8.51E-04            |

Continued on next page...

| <b>v'</b> | <b>v' (inner)</b> | <b>E(v') (cm<sup>-1</sup>)</b> | <b>FCF v'' = 35</b> | <b>FCF v'' = 36</b> |
|-----------|-------------------|--------------------------------|---------------------|---------------------|
| 119       | 119               | 27438.59                       | 6.66E-04            | 3.15E-04            |
| 120       | 120               | 27457.8                        | 1.19E-05            | 9.95E-07            |
| 121       | 121               | 27476.57                       | 4.79E-04            | 4.30E-04            |
| 122       | 122               | 27494.89                       | 0.00163             | 0.00113             |
| 123       | 123               | 27512.72                       | 0.00186             | 0.0011              |
| 124       | 124               | 27530.04                       | 7.12E-04            | 3.04E-04            |
| 125       | 125               | 27546.82                       | 1.92E-05            | 6.89E-05            |
| 126       | 126               | 27563.03                       | 0.00133             | 0.00105             |
| 127       | 127               | 27578.65                       | 0.00269             | 0.00169             |
| 128       | 128               | 27593.66                       | 0.00145             | 6.73E-04            |
| 129       | 129               | 27608.05                       | 3.14E-06            | 5.96E-05            |
| 130       | 130               | 27621.82                       | 0.00205             | 0.00161             |
| 131       | 131               | 27634.95                       | 0.00376             | 0.00223             |
| 132       | 132               | 27647.49                       | 0.00108             | 3.61E-04            |
| 133       | 133               | 27659.45                       | 6.01E-04            | 7.51E-04            |
| 134       | 134               | 27670.83                       | 0.00467             | 0.00319             |
| 135       | 135               | 27681.68                       | 0.00371             | 0.00175             |
| 136       | 136               | 27692.06                       | 1.19E-05            | 7.09E-05            |
| 137       | 137               | 27701.95                       | 0.00377             | 0.00313             |
| 138       | 138               | 27711.41                       | 0.00686             | 0.00389             |
| 139       | 139               | 27720.49                       | 0.00189             | 4.63E-04            |
| 143       | 140               | 27729.21                       | 8.21E-04            | 0.00136             |
| 146       | 141               | 27737.64                       | 0.00703             | 0.00518             |
| 150       | 142               | 27745.8                        | 0.00789             | 0.00393             |
| 153       | 143               | 27753.71                       | 0.00196             | 3.05E-04            |
| 157       | 144               | 27761.42                       | 4.81E-04            | 0.00132             |
| 160       | 145               | 27768.92                       | 0.00595             | 0.00522             |
| 164       | 146               | 27776.26                       | 0.00992             | 0.00588             |
| 167       | 147               | 27783.45                       | 0.0072              | 0.00268             |
| 171       | 148               | 27790.5                        | 0.00181             | 9.52E-05            |
| 175       | 149               | 27797.42                       | 1.30E-04            | 0.00117             |
| 178       | 150               | 27804.22                       | 0.00372             | 0.00456             |
| 182       | 151               | 27810.9                        | 0.00888             | 0.00676             |
| 186       | 152               | 27817.49                       | 0.0111              | 0.0059              |
| 190       | 153               | 27823.96                       | 0.00895             | 0.00297             |
| 195       | 154               | 27830.3                        | 0.00417             | 4.10E-04            |
| 200       | 155               | 27836.52                       | 4.47E-04            | 3.67E-04            |
| 205       | 156               | 27842.6                        | 8.03E-04            | 0.00319             |
| 211       | 157               | 27848.53                       | 0.00577             | 0.00717             |
| 219       | 158               | 27854.28                       | 0.0131              | 0.00961             |

Table 2: Franck-Condon Factors from the  $a^3\Sigma_u^+$  state to the outer well of the  $7p^3\Sigma_g^+$  state. Here,  $v'$  is the vibrational quantum number for the full potential, and  $v'$  (outer) is the numbering for the outer well alone.

| $v'$ | $v'$ (outer) | $E(v')$ ( $\text{cm}^{-1}$ ) | FCF $v'' = 35$ | FCF $v'' = 36$ |
|------|--------------|------------------------------|----------------|----------------|
| 140  | 0            | 27721.84                     | 0.0438         | 0.387          |
| 141  | 1            | 27725.27                     | 0.0136         | 0.00485        |
| 142  | 2            | 27728.65                     | 0.0315         | 0.14           |
| 144  | 3            | 27732.03                     | 0.0202         | 0.00432        |
| 145  | 4            | 27735.35                     | 0.0309         | 0.0716         |
| 147  | 5            | 27738.66                     | 0.0243         | 0.0023         |
| 148  | 6            | 27741.9                      | 0.0308         | 0.038          |
| 149  | 7            | 27745.13                     | 0.0266         | 7.78E-04       |
| 151  | 8            | 27748.32                     | 0.0309         | 0.0188         |
| 152  | 9            | 27751.48                     | 0.0278         | 5.23E-05       |
| 154  | 10           | 27754.59                     | 0.0299         | 0.00819        |
| 155  | 11           | 27757.67                     | 0.0272         | 1.63E-04       |
| 156  | 12           | 27760.72                     | 0.028          | 0.00269        |
| 158  | 13           | 27763.73                     | 0.0258         | 9.42E-04       |
| 159  | 14           | 27766.73                     | 0.0258         | 3.59E-04       |
| 161  | 15           | 27769.67                     | 0.0242         | 0.00215        |
| 162  | 16           | 27772.57                     | 0.0236         | 4.51E-05       |
| 163  | 17           | 27775.44                     | 0.0217         | 0.00354        |
| 165  | 18           | 27778.28                     | 0.0206         | 8.06E-04       |
| 166  | 19           | 27781.07                     | 0.0186         | 0.00492        |
| 168  | 20           | 27783.83                     | 0.0174         | 0.00206        |
| 169  | 21           | 27786.54                     | 0.0156         | 0.00615        |
| 170  | 22           | 27789.21                     | 0.0144         | 0.00345        |
| 172  | 23           | 27791.83                     | 0.0126         | 0.00709        |
| 173  | 24           | 27794.42                     | 0.0113         | 0.00465        |
| 174  | 25           | 27796.98                     | 0.00971        | 0.0076         |
| 176  | 26           | 27799.48                     | 0.00831        | 0.00534        |
| 177  | 27           | 27801.94                     | 0.00703        | 0.00769        |
| 179  | 28           | 27804.36                     | 0.00583        | 0.00577        |
| 180  | 29           | 27806.72                     | 0.00469        | 0.00738        |
| 181  | 30           | 27809.04                     | 0.00374        | 0.00579        |
| 183  | 31           | 27811.32                     | 0.00284        | 0.00677        |
| 184  | 32           | 27813.56                     | 0.00211        | 0.0054         |
| 185  | 33           | 27815.75                     | 0.00146        | 0.0059         |
| 187  | 34           | 27817.88                     | 9.60E-04       | 0.00471        |

Continued on next page...

| <b>v'</b> | <b>v' (outer)</b> | <b>E(v') (cm<sup>-1</sup>)</b> | <b>FCF v'' = 35</b> | <b>FCF v'' = 36</b> |
|-----------|-------------------|--------------------------------|---------------------|---------------------|
| 188       | 35                | 27819.96                       | 5.67E-04            | 0.00488             |
| 189       | 36                | 27821.99                       | 2.90E-04            | 0.00395             |
| 191       | 37                | 27824.01                       | 1.03E-04            | 0.00387             |
| 192       | 38                | 27825.96                       | 1.27E-05            | 0.00307             |
| 193       | 39                | 27827.85                       | 7.87E-06            | 0.00282             |
| 194       | 40                | 27829.69                       | 7.82E-05            | 0.0022              |
| 196       | 41                | 27831.47                       | 2.15E-04            | 0.00195             |
| 197       | 42                | 27833.22                       | 4.05E-04            | 0.00145             |
| 198       | 43                | 27834.89                       | 6.28E-04            | 0.00118             |
| 199       | 44                | 27836.49                       | 8.74E-04            | 8.32E-04            |
| 201       | 45                | 27838.03                       | 0.00115             | 6.36E-04            |
| 202       | 46                | 27839.55                       | 0.00145             | 4.12E-04            |
| 203       | 47                | 27840.99                       | 0.00168             | 2.60E-04            |
| 204       | 48                | 27842.35                       | 0.00197             | 1.39E-04            |
| 206       | 49                | 27843.67                       | 0.00221             | 6.48E-05            |
| 207       | 50                | 27844.94                       | 0.00246             | 1.68E-05            |
| 208       | 51                | 27846.15                       | 0.00264             | 3.79E-07            |
| 209       | 52                | 27847.29                       | 0.00279             | 7.79E-06            |
| 210       | 53                | 27848.34                       | 0.00281             | 3.11E-05            |
| 212       | 54                | 27849.34                       | 0.00292             | 6.98E-05            |
| 213       | 55                | 27850.28                       | 0.00301             | 1.18E-04            |
| 214       | 56                | 27851.17                       | 0.00291             | 1.64E-04            |
| 215       | 57                | 27851.97                       | 0.00277             | 2.03E-04            |
| 216       | 58                | 27852.69                       | 0.00263             | 2.38E-04            |
| 217       | 59                | 27853.35                       | 0.00249             | 2.66E-04            |
| 218       | 60                | 27853.94                       | 0.00236             | 2.89E-04            |
| 220       | 61                | 27854.49                       | 0.00227             | 3.18E-04            |
| 221       | 62                | 27854.97                       | 0.00192             | 2.95E-04            |
| 222       | 63                | 27855.37                       | 0.00171             | 2.84E-04            |
| 223       | 64                | 27855.75                       | 0.00167             | 2.97E-04            |
| 224       | 65                | 27856.08                       | 0.00138             | 2.60E-04            |
| 225       | 66                | 27856.35                       | 0.00114             | 2.26E-04            |
| 226       | 67                | 27856.59                       | 0.00107             | 2.20E-04            |
| 227       | 68                | 27856.76                       | 6.56E-04            | 1.40E-04            |
| 228       | 69                | 27856.89                       | 6.03E-04            | 1.31E-04            |
| 229       | 70                | 27857                          | 4.57E-04            | 1.01E-04            |
| 230       | 71                | 27857.09                       | 3.69E-04            | 8.30E-05            |
| 231       | 72                | 27857.15                       | 2.82E-04            | 6.41E-05            |
| 232       | 73                | 27857.2                        | 1.94E-04            | 4.44E-05            |
